# Supplementary material for: Propagation of weakly advantageous mutations in cancer cell population
Source: arXiv:2302.06573 ancillary file (2024-02-23)
Supplement: Supplementary file 1 [file Mutation_Waves_in_cacer_cells___Appendix.pdf]

# Propagation of weakly advantageous mutations in cancer cell population - Supporting information

Andrzej Polanski<sup>1</sup>, Mateusz Kania<sup>1</sup>, Jarosław Gil<sup>1</sup>, Wojciech Łabaj<sup>2</sup>, Ewa Lach<sup>1</sup>, Agnieszka Szczęśna<sup>1</sup>,

**1** Department of Computer Graphics, Vision and Digital Systems, Silesian University of Technology, Akademicka 16, 44-100 Gliwice, Poland

**2** Department of Data Science and Engineering, Silesian University of Technology, Akademicka 16, 44-100 Gliwice, Poland

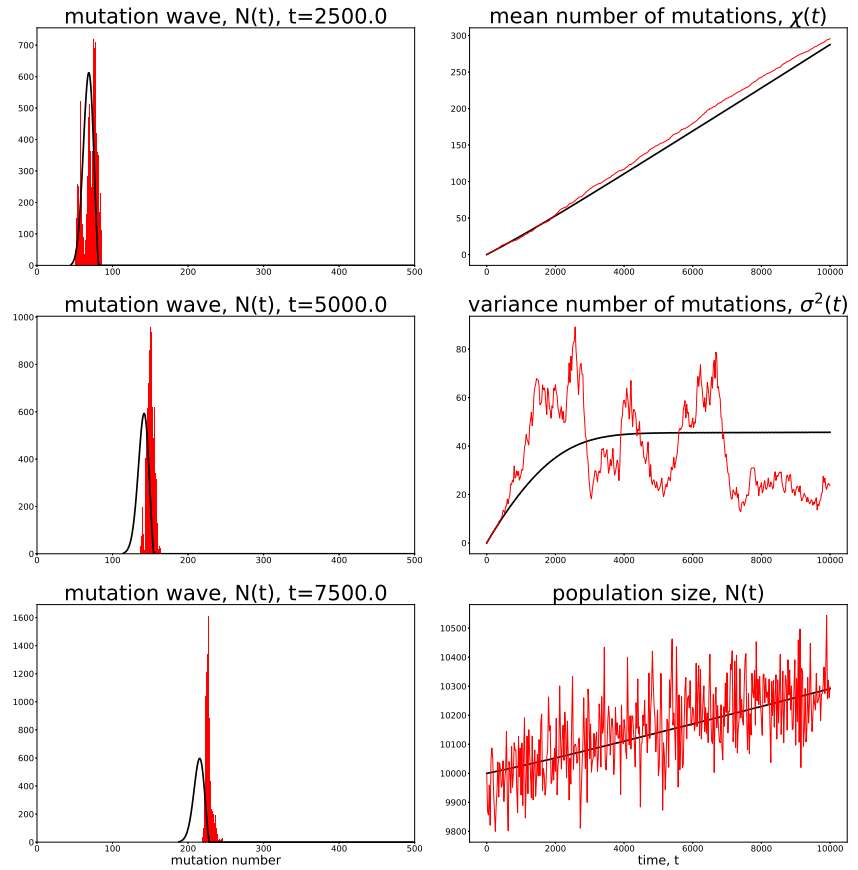

**Figure S1.** Simulation results. Black color corresponds to deterministic results, red color to stochastic simulation. Results includes moving mutation wave (left side) in three different time points and population statistics (right side) - mean number of mutations, variance number of mutations and population size changes in time.

**Table S1.** Parameters corresponding to simulation results showed in Figure S1.

| Parameter                                                      | Value  |
|----------------------------------------------------------------|--------|
| Cancer cells population size                                   | 10 000 |
| Population capacity parameter                                  | 10 000 |
| Simulation steps                                               | 10 000 |
| Tau step                                                       | 0.0050 |
| Probability of acquiring mutation in cell division             | 0.0250 |
| Value of positive selection coefficient                        | 0.0001 |
| Exponent of the power function describing cell death intensity | 1.0000 |

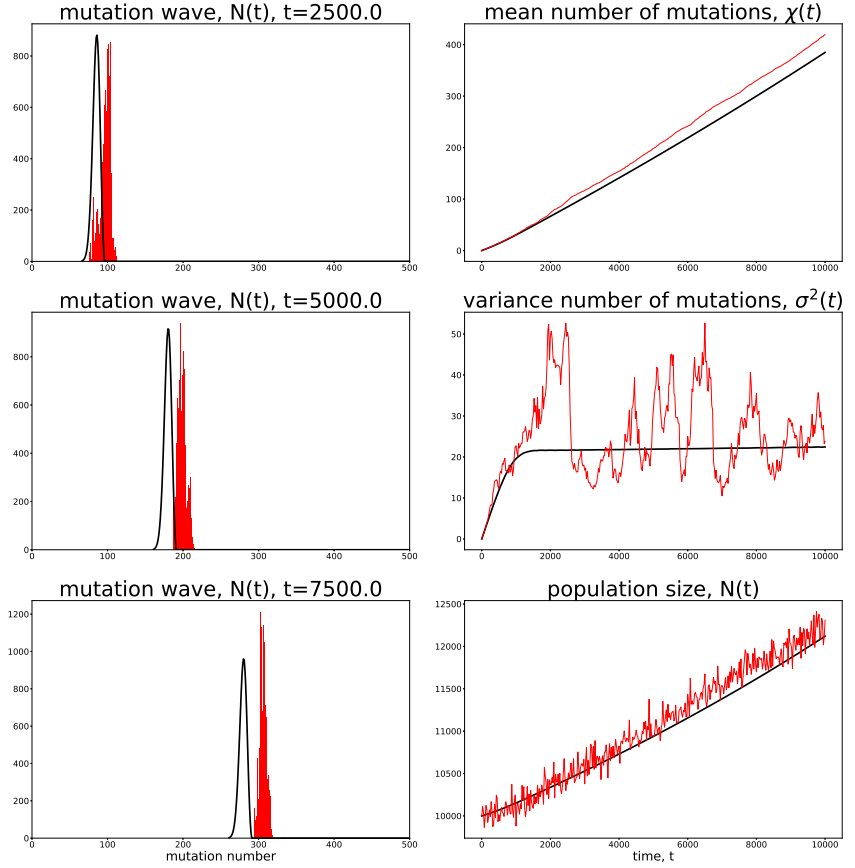

**Figure S2.** Simulation results. Black color corresponds to deterministic results, red color to stochastic simulation. Results include moving mutation wave (left side) in three different time points and population statistics (right side) - mean number of mutations, variance number of mutations and population size changes in time.

**Table S2.** Parameters corresponding to simulation results showed in Figure S2.

| Parameter                                                      | Value  |
|----------------------------------------------------------------|--------|
| Cancer cells population size                                   | 10 000 |
| Population capacity parameter                                  | 10 000 |
| Simulation steps                                               | 10 000 |
| Tau step                                                       | 0.0050 |
| Probability of acquiring mutation in cell division             | 0.0250 |
| Value of positive selection coefficient                        | 0.0005 |
| Exponent of the power function describing cell death intensity | 1.0000 |

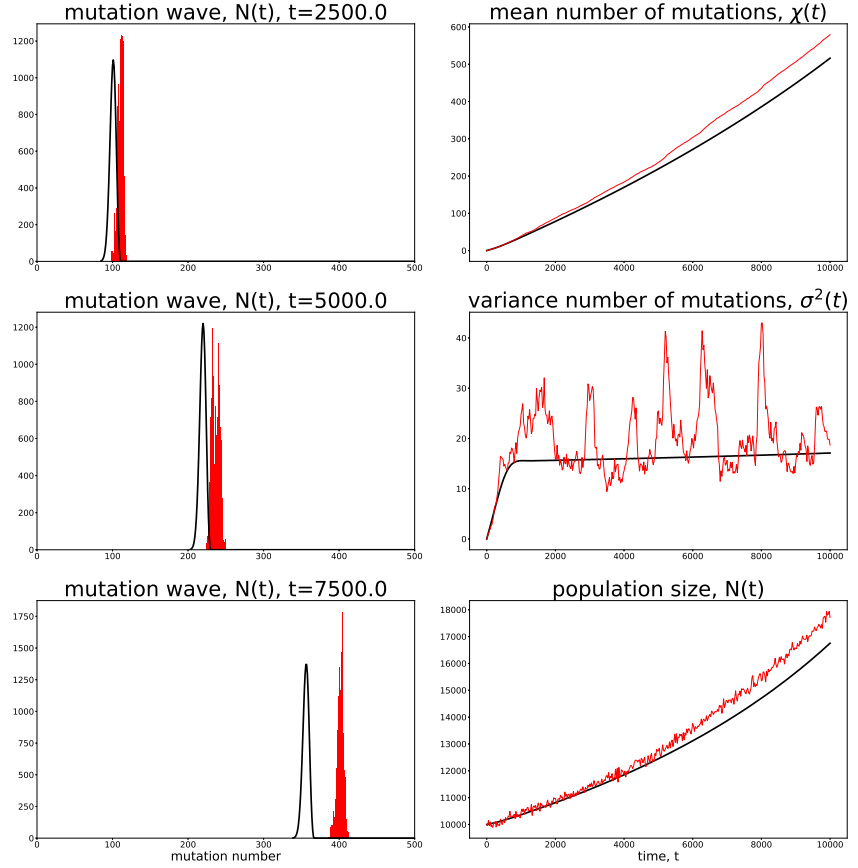

**Figure S3.** Simulation results. Black color corresponds to deterministic results, red color to stochastic simulation. Results include moving mutation wave (left side) in three different time points and population statistics (right side) - mean number of mutations, variance number of mutations and population size changes in time.

**Table S3.** Parameters corresponding to simulation results showed in Figure S3.

| Parameter                                                      | Value  |
|----------------------------------------------------------------|--------|
| Cancer cells population size                                   | 10 000 |
| Population capacity parameter                                  | 10 000 |
| Simulation steps                                               | 10 000 |
| Tau step                                                       | 0.0050 |
| Probability of acquiring mutation in cell division             | 0.0250 |
| Value of positive selection coefficient                        | 0.0010 |
| Exponent of the power function describing cell death intensity | 1.0000 |

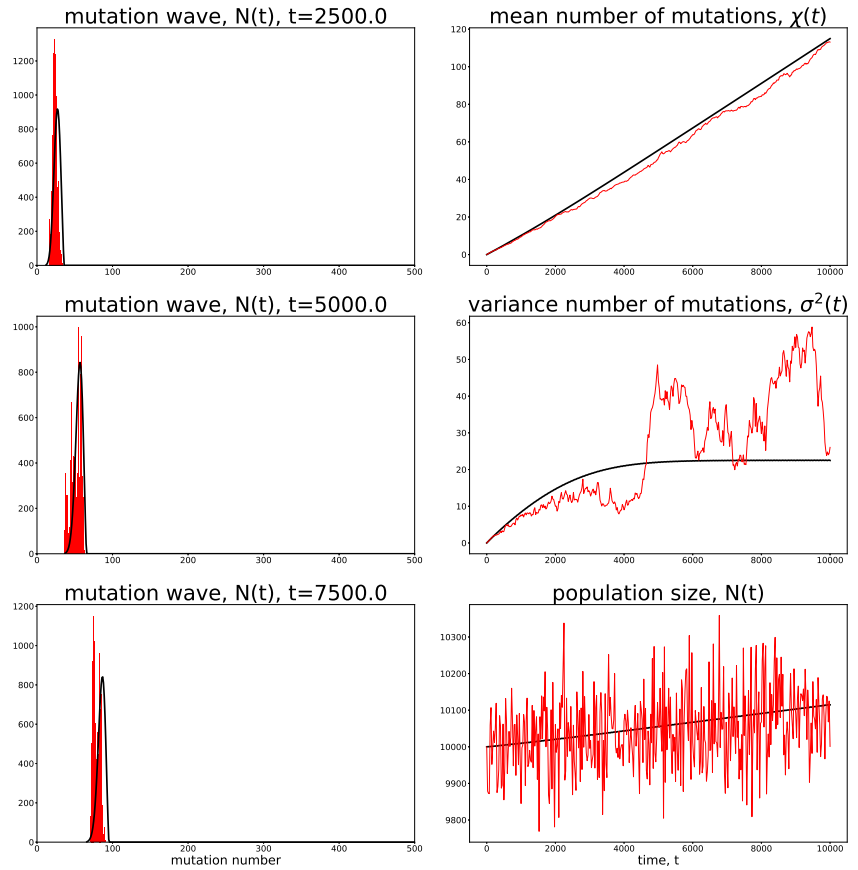

**Figure S4.** Simulation results. Black color corresponds to deterministic results, red color to stochastic simulation. Results include moving mutation wave (left side) in three different time points and population statistics (right side) - mean number of mutations, variance number of mutations and population size changes in time.

**Table S4.** Parameters corresponding to simulation results showed in Figure S4.

| Parameter                                                      | Value  |
|----------------------------------------------------------------|--------|
| Cancer cells population size                                   | 10 000 |
| Population capacity parameter                                  | 10 000 |
| Simulation steps                                               | 10 000 |
| Tau step                                                       | 0.0050 |
| Probability of acquiring mutation in cell division             | 0.0010 |
| Value of positive selection coefficient                        | 0.0001 |
| Exponent of the power function describing cell death intensity | 1.0000 |

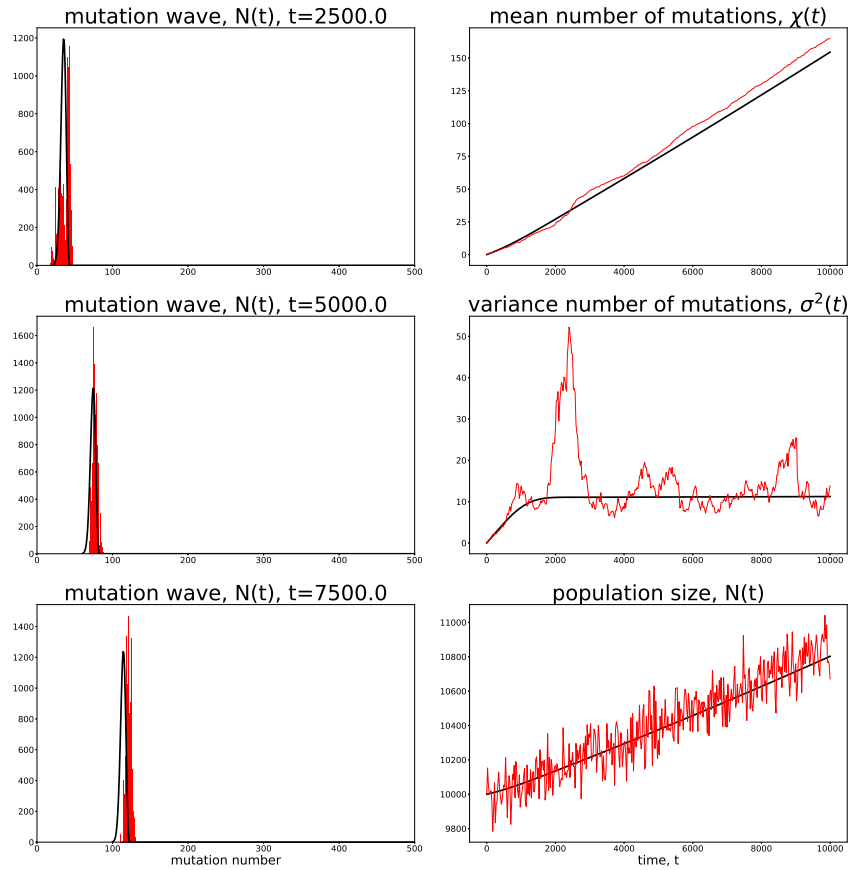

**Figure S5.** Simulation results. Black color corresponds to deterministic results, red color to stochastic simulation. Results include moving mutation wave (left side) in three different time points and population statistics (right side) - mean number of mutations, variance number of mutations and population size changes in time.

**Table S5.** Parameters corresponding to simulation results showed in Figure S5.

| Parameter                                                      | Value  |
|----------------------------------------------------------------|--------|
| Cancer cells population size                                   | 10 000 |
| Population capacity parameter                                  | 10 000 |
| Simulation steps                                               | 10 000 |
| Tau step                                                       | 0.0050 |
| Probability of acquiring mutation in cell division             | 0.0010 |
| Value of positive selection coefficient                        | 0.0005 |
| Exponent of the power function describing cell death intensity | 1.0000 |

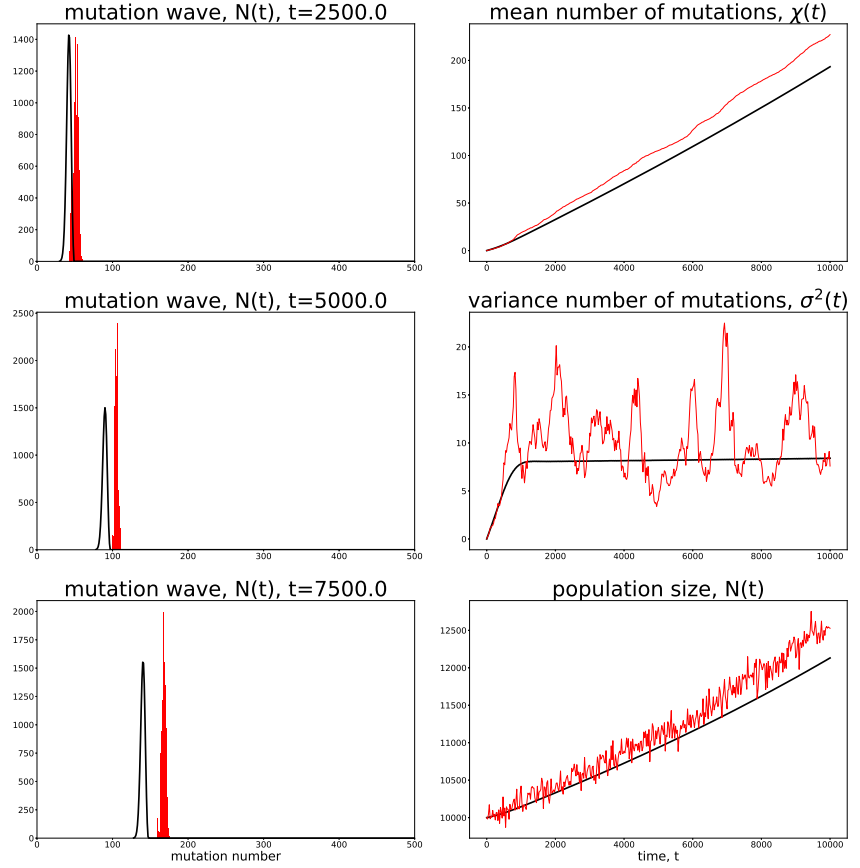

**Figure S6.** Simulation results. Black color corresponds to deterministic results, red color to stochastic simulation. Results includes moving mutation wave (left side) in three different time points and population statistics (right side) - mean number of mutations, variance number of mutations and population size changes in time.

**Table S6.** Parameters corresponding to simulation results showed in Figure S6.

| Parameter                                                      | Value  |
|----------------------------------------------------------------|--------|
| Cancer cells population size                                   | 10 000 |
| Population capacity parameter                                  | 10 000 |
| Simulation steps                                               | 10 000 |
| Tau step                                                       | 0.0050 |
| Probability of acquiring mutation in cell division             | 0.0010 |
| Value of positive selection coefficient                        | 0.0010 |
| Exponent of the power function describing cell death intensity | 1.0000 |

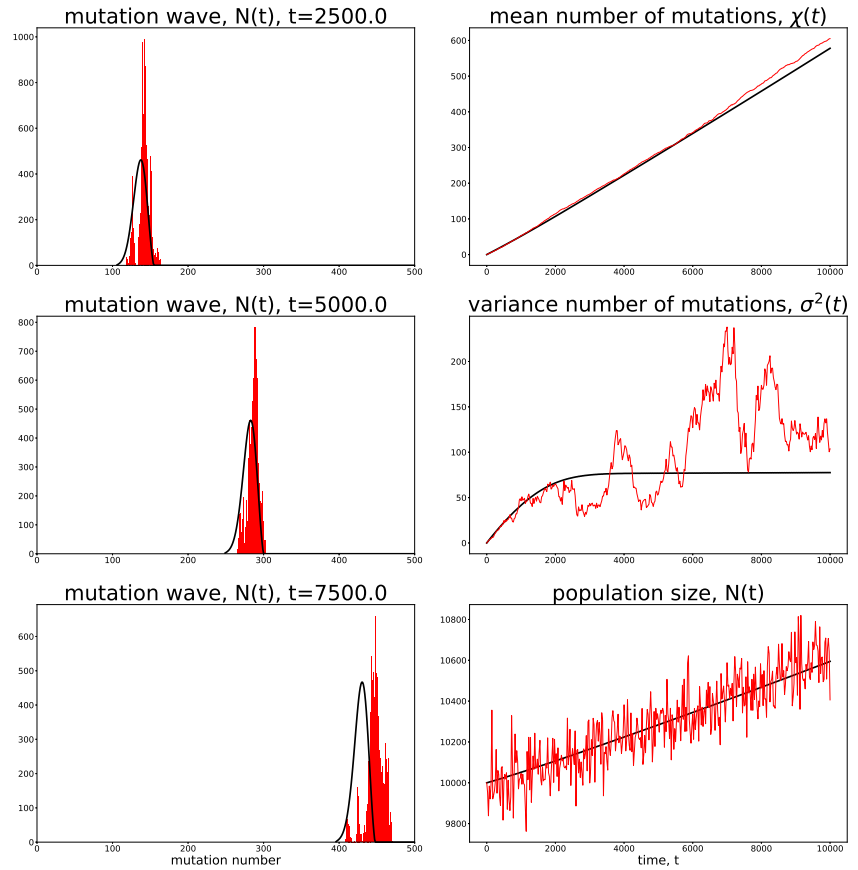

**Figure S7.** Simulation results. Black color corresponds to deterministic results, red color to stochastic simulation. Results include moving mutation wave (left side) in three different time points and population statistics (right side) - mean number of mutations, variance number of mutations and population size changes in time.

**Table S7.** Parameters corresponding to simulation results showed in Figure S7.

| parameter                                                      | value  |
|----------------------------------------------------------------|--------|
| Cancer cells population size                                   | 10 000 |
| Population capacity parameter                                  | 10 000 |
| Simulation steps                                               | 10 000 |
| Tau step                                                       | 0.0050 |
| Probability of acquiring mutation in cell division             | 0.0500 |
| Value of positive selection coefficient                        | 0.0001 |
| Exponent of the power function describing cell death intensity | 1.0000 |

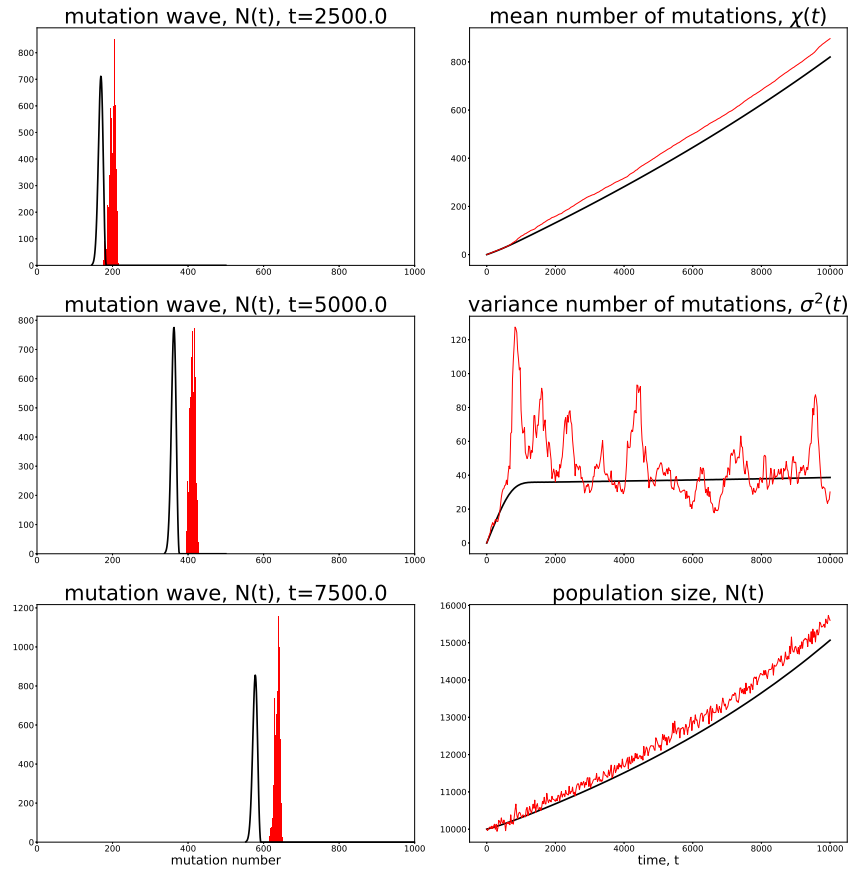

**Figure S8.** Simulation results. Black color corresponds to deterministic results, red color to stochastic simulation. Results include moving mutation wave (left side) in three different time points and population statistics (right side) - mean number of mutations, variance number of mutations and population size changes in time.

**Table S8.** Parameters corresponding to simulation results showed in Figure S8.

| Parameter                                                      | Value  |
|----------------------------------------------------------------|--------|
| Cancer cells population size                                   | 10 000 |
| Population capacity parameter                                  | 10 000 |
| Simulation steps                                               | 10 000 |
| Tau step                                                       | 0.0050 |
| Probability of acquiring mutation in cell division             | 0.0500 |
| Value of positive selection coefficient                        | 0.0005 |
| Exponent of the power function describing cell death intensity | 1.0000 |

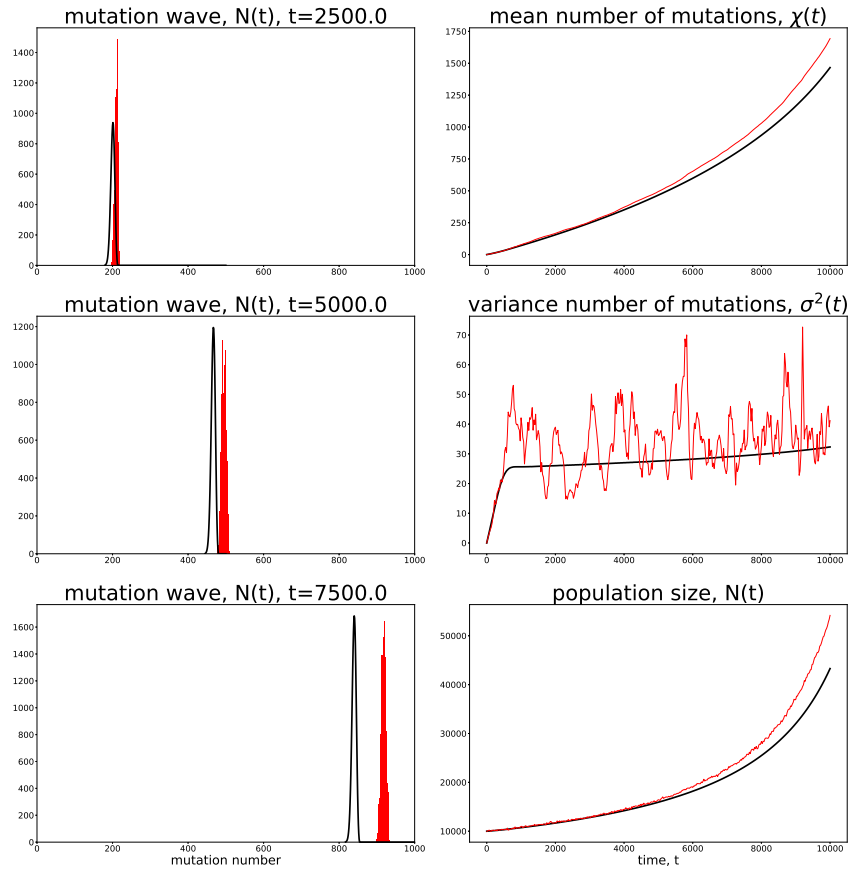

**Figure S9.** Simulation results. Black color corresponds to deterministic results, red color to stochastic simulation. Results include moving mutation wave (left side) in three different time points and population statistics (right side) - mean number of mutations, variance number of mutations and population size changes in time.

**Table S9.** Parameters corresponding to simulation results showed in Figure S9.

| Parameter                                                      | Value  |
|----------------------------------------------------------------|--------|
| Cancer cells population size                                   | 10 000 |
| Population capacity parameter                                  | 10 000 |
| Simulation steps                                               | 10 000 |
| Tau step                                                       | 0.0050 |
| Probability of acquiring mutation in cell division             | 0.0500 |
| Value of positive selection coefficient                        | 0.0010 |
| Exponent of the power function describing cell death intensity | 1.0000 |

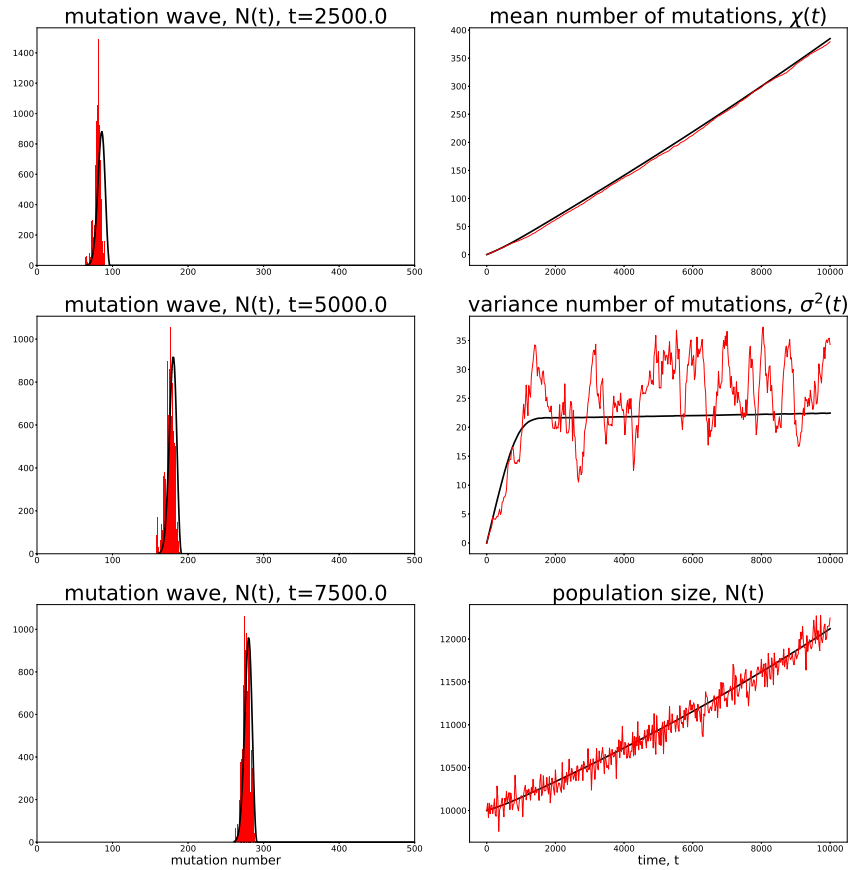

**Figure S10.** Simulation results. Black color corresponds to deterministic results, red color to stochastic simulation. Results include moving mutation wave (left side) in three different time points and population statistics (right side) - mean number of mutations, variance number of mutations and population size changes in time.

**Table S10.** Parameters corresponding to simulation results showed in Figure S10.

| Parameter                                                      | Value  |
|----------------------------------------------------------------|--------|
| Cancer cells population size                                   | 10 000 |
| Population capacity parameter                                  | 10 000 |
| Simulation steps                                               | 10 000 |
| Tau step                                                       | 0.0500 |
| Probability of acquiring mutation in cell division             | 0.0250 |
| Value of positive selection coefficient                        | 0.0005 |
| Exponent of the power function describing cell death intensity | 1.0000 |
